# Supplementary material for: DeVLBert: Learning Deconfounded Visio-Linguistic Representations
Source: arXiv:2008.06884 source file (2020-10-02)
Supplement: Supplementary file 1 [file 7.Appendix.tex]

\section{Appendix}
\label{sec:appendix}

\subsection{Details on the Experimental Setup and Hyperparameters}

% Batch Normalization\cite{Ioffe_Szegedy_2015}
% We apply Dropout on the activation output to improve generalization.

%For information propagation module, we apply Batch Normalization\cite{Ioffe_Szegedy_2015} before the activation function and dropout on the activation output to improve generalization. We also add dropout on the input of RNN decoder.

%Batch Normalization\cite{Ioffe_Szegedy_2015}

%Since we have three input graphs, we progressively perform information propagation for individual graphs and aggregated graphs, which is obtained by the global-local aggregation module, as depicted in Fig \ref{fig:GLA}. In practice, we firstly aggregate the content graph and the attribute graph into the attribute-content (AC) graph and finally obtain the video-attribute-content (VAC) graph by further aggregate the video graph. The VAC graph conveys the necessary cues about the styles, patterns and designs of the product. The detailed model structure and dimension setup can be found in Figure [TOREF].

\vpara{Hyper-parameter Configuration} The parameter setup of \textit{granular level interaction modeling} process is shown in Figure \ref{fig:granular-level}. During training, the batch size is set to 64 and we use Adam optimizer \cite{Kingma_Ba_2015} with the setting $\beta _ { 1 } = 0.9 , \beta _ { 2 } = 0.999,  \mathrm{weight decay} = 1 \times 10 ^ {-4} \text { and } \epsilon = 1 \times 10 ^ { - 8 }$. Learning rate is $4 \times 10 ^ {-4}$. We employ dropout rate of 0.2 and batch normalization after graph information propgation. We also applied a dropout rate of 0.5 for RNNs and linear layers as regularization.  The hidden size of both story-line summarization RNN and decoder RNN is set to 512. The loss weight $\lambda_{gc}$ is set to 0.1.
At the inference stage, we use the greedy strategy to generate the final title.

%--------------------------------fig-------------------------
\begin{figure}[!h] \begin{center}
    \includegraphics[width=\columnwidth]{./figures/Granular-Level.pdf}
    \caption{
    Architecture and parameter configuration of granular-level interaction modeling process.
	}
%\vspace{-0.4cm}
\label{fig:granular-level}
\end{center} \end{figure}
%--------------------------------fig end--------------------

%During Training:
%BatchSize
%Optimizer params |  learning rate 
%Dropout BatchNorm
%loss params
%
%During Inference:
%Greedy

% 详细模型图

%--------------------------------fig-------------------------
\begin{figure}[!t] \begin{center}
    \includegraphics[width=\columnwidth]{./figures/example.pdf}
    \caption{
    A <video, comment, attributes, title> quadruple data sample in T-VTD.
	}
%\vspace{-0.4cm}
\label{fig:example}
\end{center} \end{figure}
%--------------------------------fig end--------------------

\vpara{Hardware \& Software Configuration }
The experiments are conducted on a Linux server equipped with an Intel(R) Xeon(R) CPU E5-2690 v4 @ 2.60GHz, 512GB RAM and 1 NVIDIA Titan V GPU.
All models are implemented in PyTorch \citep{paszke2017automatic} of version 1.2.0, pytorch-geometric \cite{Fey_Lenssen_2019} of version 1.3.2 and Python 3.6.
We'll soon release the main code of \Our for reproduction and further development.

%--------------------------------table-------------------------

\begin{table*}[t]
%\begin{strip}
\centering
\setlength{\tabcolsep}{7.5pt}
\setlength\doublerulesep{0.5pt}
%\footnotesize  
%\small
\begin{tabular}{l|cccccc}

%\cline{1-9}
% <<<

\multicolumn{1}{c|}{Dataset} &    Context      &   \#Video    &   \#Sentence & \#Word & \#Vocabulary  &  Total Duration(hrs)   \\
\hline \hline

MSVD \cite{Chen_Dolan_2011}            & multi-category          &    1,970        &    70,028 & 607,339  & 13,010    & 5.3           \\
%\hline 

%

YouCook \cite{Das_Xu_Doell_Corso_2013}  & cooking     &  88  &  2,668  &   42,457  & 2,711  &  2.3 \\
%\hline
TACos  \cite{Regneri_Rohrbach_Wetzel_Thater_Schiele_Pinkal_2013}   &  cooking    &  123  &  18,227  &  146,771  & 28,292 &  15.9
        \\
%\hline
TACos M-L \cite{Rohrbach_Rohrbach_Qiu_Friedrich_Pinkal_Schiele_2014}  &  cooking  & 185   &  14,105  &  52,593  & - &  27.1
\\
%\hline
MPII-MD \cite{Rohrbach_Rohrbach_Tandon_Schiele_2015}  &  movie      &  94  &  68,375  &  653,467   & 24,549 &  73.6
\\
%\hline
M-VAD \cite{Torabi_Pal_Larochelle_Courville_2015}  &  movie        &  92  &  55,905   &  519,933   & 18,269  &  84.6
\\
VTW \cite{Torabi_Pal_Larochelle_Courville_2015}  &  multi-category        &  18,100  &  44,603   &  -   & 23,059  &  213.2
\\

MSR-VTT \cite{Zeng_Chen_Niebles_Sun_2016}  &  multi-category  & 7,180    & 200,000  &  1,856,523    & 29,316 &  41.2
\\
Charades \cite{Sigurdsson_Varol_Wang_Farhadi_Laptev_Gupta_2016}  &  human     &  9,848  & 27,847  & - & -  &  82.01
%\\
%Bilibili  &  live      & 2,361    & 895,929  & 4,860,246 & -  &   113.84
\\
\hline
\hline
T-VTD  &  e-commerce   & 90,000    & 180,000  & 3,878,436 & 68,232  &  755.73
\\
\hline
%\\
%\\

\end{tabular}
\caption{
Comparison between T-VTD with benchmark video captioning datasets, considering various capacity indicators.. 
}
%\vspace{-0.4cm}
\label{table:Data}
\end{table*}

%---------------------------table end-------------------------

\subsection{Additional Details on the Dataset } \label{sub:data}
The summarized statistics of T-VTD and comparisons with other frequently used benchmark video captioning datasets are shown in Figure \ref{table:Data}. Specifically, T-VTD contains 90000 videos with a total length of 755.73 hours, which is much larger than current datasets. As for natural language data, T-VTD has totally 3,878,436 words (in titles and comments) with a vocabulary of 68232. The nature of abundant vocabulary and little repetitive information poses a direct challenge to fully understand the semantic information and avoid obtaining high scores just by overfitting to some biases. We summary the statistics of video durations in our dataset in Table \ref{table:videoduration}. The video durations in our dataset are mainly 15-30s, with an average video length around 30.23s. The longest video can reach 600 seconds (about 10 minutes). As shown in Table \ref{table:titlecontent} and \ref{table:attributes}, the average length of elements in the titles, comments and attributes are 6.6, 36.49 and 17.54, respectively. The vocabulary size is 27,976 for video titles and 59,109 for narrative comments. There are 81 different attribute-key types and 266,648 different attribute-value types, \ie, the vocabulary size of human-nameable attributes. A real case in our dataset is shown in Figure \ref{fig:example}. It can be seen that the comment sentences mainly narrate the preference for different aspects of products. Although the attributes of associated products structurally specify the human-nameable qualities of the products, these attributes can be noisy since they may cover all possible choices (such as different colors) and not exactly the product in the video. Models are required to fully understand the video rather than simply distill information from the attributes or the comment.

%30.23

%--------------------------------table-------------------------

\begin{table}[!t]
\centering
\setlength{\tabcolsep}{5.5pt}
\setlength\doublerulesep{0.5pt}
\begin{tabular}{l|ccc}

%\cline{1-9}
% <<<

  &    avg\_len      &   total\_len    &    vocab  \\
\hline \hline

%\hline
title   &  6.6  & 594,279    & 27,976
\\
%\hline
comment   &  36.49  & 3,284,157    & 59,109
\\

\hline

\end{tabular}
\caption{
    Basic statistics of titles and comments in T-VTD.
}
\label{table:titlecontent}
\end{table}

%---------------------------table end-------------------------
%[TODO]

\subsection{Details on Data Pre-processing} \label{sub:id}

For text pre-processing, we remove the punctuations and tokenize sentences using Jieba Chinese Tokenizer \footnote{https://github.com/fxsjy/jieba}. Our vocabulary contains all attributes values, comment tokens and ground-truth title tokens. Since the real-world text data is noised and many expressions can be confusing or meaningless, such as brands and homophonic words. We roughly filter them by replacing low-frequency tokens (less than 50) with the special token $<unk>$, resulting in 6347 tokens in total. The length limitations for title, comment and attributes are 12, 50 and 15, respectively. Text with number of tokens more than the corresponding limitation will be truncated. We add a special $<sos>$ token as the first word for the title and a $<eos>$ at the end. When the $<sos>$ token is predicted in the decoding stage, the generation will be terminated.

For video processing, we first uniformly sample 30 frames per video. For landmark feature extraction, we extract the product area using internal product detector for all sampled frames. Then we use the pre-trained landmark detector \footnote{https://github.com/fdjingyuan/Deep-Fashion-Analysis-ECCV2018} provided by \cite{liu2018deep}. Specifically, the backbone model $VGG16$ takes each frame as input and output the activations of shape $512 \times 7 \times 7$ from layer \textit{pooled\_5}. This feature map is forwarded to the landmark decoder, which produce the landmark-oriented features of shape $64 \times 14 \times 14$ and the mask-like landmark maps of shape $8 \times 56 \times 56$, \ie, 8 landmarks maps of shape $\times 56 \times 56$ each. We downsampled each landmark map to have the same width and height as the landmark-oriented features. Deriving from the observation that intermediate feature map and emergent patterns are highly correlated, we normalize each landmark map as weights using softmax and compute weighted sum over the landmark-oriented features as the landmark feature.

%--------------------------------table-------------------------

\begin{table}[!t]
\centering
\setlength{\tabcolsep}{3.5pt}
\setlength\doublerulesep{0.5pt}
\begin{tabular}{l|cccccc}

%\cline{1-9}
% <<<

  &    average  & min  & Q1   &   median   &  Q3 & max  \\
\hline \hline

%\hline
video duration (s)  & 30.23  &  1.5   & 15.72  & 23.56    & 32.2  & 600.08
\\

\hline

\end{tabular}
\caption{
    Statistics of the video duration. (Q1 denotes the lower quartile and Q3 denotes the upper quartile.)
}
\label{table:videoduration}
\end{table}

%---------------------------table end-------------------------

%%--------------------------------fig-------------------------
%\begin{figure}[!t] \begin{center}
%    \includegraphics[width=\columnwidth]{./figures/video_distribution.png}
%    \caption{
%    Video length distribution in T-VTD.
%	}
%%\vspace{-0.4cm}
%\label{fig:videolen}
%\end{center} \end{figure}
%%--------------------------------fig end--------------------

For frame-level feature extraction, we use the same model as landmark feature extraction and obtain the activations of shape $128 \times 7 \times 7$ from layer \textit{conv4} for each frame. We use the global average pooling result as the frame feature.

The dataset we use for training is a subset (84394 samples) of the released dataset (90000 samples) due to the the data pre-processing (mainly the low-frequency words removal procedure) after which many words in the comment and elements in the attributes set will be replaced by $<unk>$. Specifically, we remove the following 3 kinds of samples: 1) sample with less than 2 non-$<unk>$ elements (\ie, where will be no edges in the graph) in the attributes set. 2) sample with 0 non-$<unk>$ words in the title. 3) sample with less than 11 non-$<unk>$ nodes in or less than 5 edges in the narrative comment graph. Overall, we mainly remove samples with little information within either one kind of fact (narrative comment or human-nameable attributes) or the ground truth title to make the data more reliable.

We randomly split the whole dataset by train 65\%, validation 5\% and test 30\%, resulting in 54856 samples for training, 4220 samples for validation and 25318 samples for testing.

%--------------------------------table-------------------------

\begin{table}[!t]
\centering
\setlength{\tabcolsep}{2.5pt}
\setlength\doublerulesep{0.5pt}
\begin{tabular}{l|ccccc}

%\cline{1-9}
% <<<

  &    \multirow{2}{*}{avg\_num}      &   total\_num   &    total\_num  &  vocab & vocab  \\ & &  of keys & of values & of keys & of values  \\
\hline \hline

%\hline
attributes   &  17.54  &  1,578,777    &  2,604,904  &  81 & 266,648
\\

\hline

\end{tabular}
\caption{
    Basic statistics of attributes in T-VTD.
}
\label{table:attributes}
\end{table}

%---------------------------table end-------------------------

% In other words, each pixel on the normalized landmark map represent the probability the  feature of the sample

% For image classification networks, Bau et al. (2017) has observed that many units can approximately locate emergent object classes when the units are upsampled and thresholded.

%\subsection{More Cases} \label{sub:case}
%[TODO] may not include this?
